# Supplementary material for: Multimodal Filesystem Memory For Long-Horizon Embodied Agents
Source: arXiv:2610.22686 source file (2026-10-28)
Supplement: Supplementary file 1 [file app_additional_examples_old.tex]

\section{Additional Examples}
\Cref{fig:tech-tree} shows that MFM enables continued progress toward the Ender Dragon beyond the milestones reached by the baselines. Although VISTA obtains diamond equipment earlier, its progress subsequently plateaus, whereas MFM advances through obsidian and flint and steel to reach netherrack within the same interaction budget.

\begin{figure*}[ht]
  \centering

    \includegraphics[width=\linewidth]{figs/dragon_tech_tree_gpt-6-astra_cap36k_clean.png} 
 



  \caption{\small \textbf{Milestone progression on the Ender Dragon task with gpt-6-Astra.} Curves show progression through the Minecraft technology tree against environment steps (logarithmic scale). Under a shared 36,000-step budget, MFM reaches 16 of 24 milestones, compared with 13 for VISTA, 12 for PRO-LONG, and 6 for direct evaluation (selected single-seed runs). The vertical dashed line marks the interaction budget, and the shaded region indicates milestones no method reached.
  }
  \label{fig:tech-tree}
\end{figure*}






\begin{figure*}[ht]
  \centering
    \includegraphics[width=\linewidth]{figs/steps_per_turn_projected.pdf} 
  \caption{\small \textbf{Environment interaction per agent turn.} Rolling median of environment steps executed per agent turn over each run, across three base models (columns) on Mine Diamond from Scratch (top) and the Ender Dragon (bottom). Higher values indicate more environment interaction between successive agent turns; the vertical axis is logarithmic. Shaded regions mark intervals where MFM exceeds both VISTA and PRO-LONG, with annotations reporting the shaded fraction of each panel.
  }
  \label{fig:steps-per-turn}
\end{figure*}


\begin{figure*}[ht]
  \centering
    \begin{subfigure}[t]{0.32\textwidth}
    \centering
    \includegraphics[width=\linewidth]{figs/kicad/55f2eefb/mfm_gpt6/s009_change_symbol_ok_but_agent_notices_value.png} 
    \caption{\small Task 55f2eefb. }
    \label{fig:s009_change_symbol_ok_but_agent_notices_value}
  \end{subfigure}
  \begin{subfigure}[t]{0.32\textwidth}
    \centering
    \includegraphics[width=\linewidth]{figs/kicad/c4baee36/mfm_gpt6/s045_finished_schematic_with_48v_and_gnd_symb.png} 
    \caption{\small Task: c4baee36}
    \label{fig:s045_finished_schematic_with_48v_and_gnd_symb}
   \end{subfigure}
      \begin{subfigure}[t]{0.32\textwidth}
    \centering
    \includegraphics[width=\linewidth]{figs/kicad/b7148878/mfm_gpt6/s094_full_schematic.png} 
    \caption{\small Task: b7148878}
    \label{fig:s094_full_schematic}
   \end{subfigure}
   
  \begin{subfigure}[t]{0.32\textwidth}
    \centering
    \includegraphics[width=\linewidth]{figs/kicad/55f2eefb/vista_gpt56/s010_label_still_reads_9v_on_screen_agent_mis.png} 
    \caption{\small Task: 55f2eefb}
    \label{fig:s010_label_still_reads_9v_on_screen_agent_mis}
  \end{subfigure}
  \begin{subfigure}[t]{0.32\textwidth}
    \centering
    \includegraphics[width=\linewidth]{figs/kicad/c4baee36/vista_gpt56/s060_local_label_3_3vdc_on_the_output_net.png} 
    \caption{\small Task: c4baee36 }
    \label{fig:s060_local_label_3_3vdc_on_the_output_net}
   \end{subfigure}
   \begin{subfigure}[t]{0.32\textwidth}
    \centering
    \includegraphics[width=\linewidth]{figs/kicad/b7148878/vista_gpt56/s125_saved_done_netlist_r1_1_u2_1_u2_2_dangli.png} 
    \caption{\small Task: b7148878}
    \label{fig:s125_saved_done_netlist_r1_1_u2_1_u2_2_dangli}
   \end{subfigure}
  \caption{\small \textbf{Qualitative comparison on CUABench-KiCad.} Top: results produced by MFM. Bottom: results produced by VISTA on the same three tasks. Columns correspond to Task 55f2eefb, Task c4baee36, and Task b7148878, respectively. }
  \label{fig:kicad-tasks-different-perf}
\end{figure*}


\begin{figure*}[ht]
  \centering
  \begin{subfigure}[t]{0.5\textwidth}
    \centering
    \includegraphics[width=\linewidth]{figs/crop_examples/01_frame_640x360_step4588.jpg} 
    \caption{\small Initial observation of a pale animal.}
    \label{fig:crop-wolf-a}
  \end{subfigure}
  \hfill
  \begin{subfigure}[t]{0.34\textwidth}
    \centering
    \includegraphics[width=\linewidth]{figs/crop_examples/01_zoom_crop.png} 
    \caption{\small Zoomed-in view revealing a wolf.}
    \label{fig:crop-wolf-b}
   \end{subfigure}
   \\
  \begin{subfigure}[t]{0.5\textwidth}
    \centering
    \includegraphics[width=\linewidth]{figs/crop_examples/02_frame_640x360_step4917.jpg} 
    \caption{\small Initial observation of a possible pink sheep.}
    \label{fig:crop-sheep-a}
  \end{subfigure}
  \hfill
  \begin{subfigure}[t]{0.3\textwidth}
    \centering
    \includegraphics[width=\linewidth]{figs/crop_examples/02_zoom_crop.png} 
    \caption{\small Zoomed-in view of the sheep.}
    \label{fig:crop-sheep-b}
   \end{subfigure}
  \caption{\small Visual memory inspection for correcting perceptual errors (a–b) and resolving uncertainty (c–d).
  % \textbf{Correcting perceptual errors through visual memory inspection.} al for a sheep. By magnifying the original observation from memory, it correctly identifies the animal as a wolf and revises its plan, avoiding an unnecessary attack.
  % Agent observed a pale animal saw a sheep. By zoomed into the observation from memory, it verified that it is a wolf: do not attack, no fight, no damage. 
   % \textbf{Resolving perceptual uncertainty through visual memory inspection.} The agent is initially uncertain whether the observed animal is a pink sheep. By zooming into the original visual observation, it verifies the sheep and uses this information to guide its subsequent plan for obtaining food and wool.
  % Agent observed but was not sure if it were a pink sheep: food and wool, kill sheep, mutton -> cooked mutton. 
  }
  \label{fig:crop-wolf}
\end{figure*}

\begin{figure*}[ht]
  \centering
  \begin{subfigure}[t]{0.34\textwidth}
    \centering
    \includegraphics[width=\linewidth]{figs/crop_examples/03_frame_640x360_step884.jpg} 
    \caption{\small Earlier observation of the hole}
    \label{fig:03-a}
  \end{subfigure}
  \begin{subfigure}[t]{0.65\textwidth}
    \centering
    \includegraphics[width=\linewidth]{figs/crop_examples/03_then_now_sheet.png} 
    \caption{\small Relocating the hole using visual memory}
    \label{fig:03-then-now}
   \end{subfigure}
  \caption{\small \textbf{Memory-guided spatial relocation.} The close visual alignment between the retrieved and current views allows the agent to identify the hole’s rim and recover its precise location.
  }
  \label{fig:03}
  \vskip -0.4cm
\end{figure*}

\begin{figure*}[ht]
  \centering
  \begin{subfigure}[t]{0.34\textwidth}
    \centering
    \includegraphics[width=\linewidth]{figs/crop_examples/04_frame_640x360_step6138.jpg} 
    \caption{\small Life 1: original observation}
    \label{fig:04_frame_640x360_step6138}
  \end{subfigure}
  \begin{subfigure}[t]{0.65\textwidth}
    \centering
    \includegraphics[width=\linewidth]{figs/crop_examples/04_then_now_sheet.png} 
    \caption{\small Life 2: retrieved memory vs. current observation}
    \label{fig:04_then_now_sheet}
   \end{subfigure}
  \caption{\small \textbf{Cross-life visual memory retrieval.} Agent retrieves an observation from Life 1 and compares it against its current view in Life 2, correctly recognizing that the live bank is the entrance to Life 1’s iron mine.
  %  1's frame  (a life two generations back)	the live bank is that life's iron entrance	mine iron ore verified at step 6565, first ore of the life
  }
  \label{fig:04}
\end{figure*}

\begin{figure*}[ht]
  \centering
  \begin{subfigure}[t]{0.49\textwidth}
    \centering
    \includegraphics[width=\linewidth]{figs/crop_examples/05_frame_640x360_step1855.jpg} 
    \caption{\small Retrieved frame with incorrect viewing angle}
    \label{fig:05_frame_640x360_step1855}
  \end{subfigure}
  \begin{subfigure}[t]{0.49\textwidth}
    \centering
    \includegraphics[width=\linewidth]{figs/crop_examples/05_viewed_frame_ep_000126_step1777.png} 
    \caption{\small Re-aimed view for continued mining}
    \label{fig:05_viewed_frame_ep_000126_step1777}
   \end{subfigure}
  \caption{\small \textbf{Using visual memory to recover mining orientation.} After retrieving the previous entry’s frame, the agent recognizes that the recorded view is aimed upward rather than toward the mining face. It adjusts its view accordingly and resumes mining from the correct orientation.
  % view of the last entry's frame	the aim pointed up, not at the feet	look\_abs re-aim, level floor next turn
  }
  \label{fig:05}
\end{figure*}


Figures \ref{fig:4_erc_practice_ba34f1c3}, \ref{fig:4_erc_practice_4c913e30}, \ref{fig:4_erc_practice_5dbc9e02} show how MFM verifies its own edits on the three CUABench-KiCad tasks discussed in \Cref{sec:qualitative}. In each case, the agent follows the same three-step routine, which it first performed in an earlier task and later retrieved from episodic memory (cf. \Cref{fig:}): it inspects the schematic to confirm that component values and net labels match the specification (a), opens the Electrical Rules Checker (b), and reads the ERC report to confirm that only the expected undriven-power warnings remain and that no pins are left unconnected (c). Checking the resulting application state, rather than trusting the edit operation's "OK" response, allows MFM to catch incomplete edits that VISTA records as successful (\Cref{fig:kicad-tasks-different-perf}).

\begin{figure*}[ht]
  \centering
  \begin{subfigure}[t]{0.32\textwidth}
    \centering
    \includegraphics[width=\linewidth]{figs/kicad/4_erc_practice/ba34f1c3_step_45.png} 
    \caption{\small The label and all five nets match the design. The title and status bar confirm the schematic is saved.  }
    \label{fig:ba34f1c3_step_45}
  \end{subfigure}
  \begin{subfigure}[t]{0.32\textwidth}
    \centering
    \includegraphics[width=\linewidth]{figs/kicad/4_erc_practice/ba34f1c3_step_46.png} 
    \caption{\small ERC is open and ready; no feedback errors appear.  }
    \label{fig:ba34f1c3_step_46}
   \end{subfigure}
   \begin{subfigure}[t]{0.32\textwidth}
    \centering
    \includegraphics[width=\linewidth]{figs/kicad/4_erc_practice/ba34f1c3_step_47.png} 
    \caption{\small ERC shows only the two expected undriven-power errors, with zero warnings.  }
    \label{fig:ba34f1c3_step_47}
   \end{subfigure}
  \caption{\small  Task ba34f1c3: open ERC, dialog, results. }
  \label{fig:4_erc_practice_ba34f1c3}
\end{figure*}

\begin{figure*}[ht]
  \centering
  \begin{subfigure}[t]{0.32\textwidth}
    \centering
    \includegraphics[width=\linewidth]{figs/kicad/4_erc_practice/4c913e30_step_76.png} 
    \caption{\small The wiring matches the committed design, and the schematic is saved in the required directory. }
    \label{fig:4c913e30_step_76}
  \end{subfigure}
  \begin{subfigure}[t]{0.32\textwidth}
    \centering
    \includegraphics[width=\linewidth]{figs/kicad/4_erc_practice/4c913e30_step_77.png} 
    \caption{\small ERC is ready; no feedback errors appear.  }
    \label{fig:4c913e30_step_77}
   \end{subfigure}
   \begin{subfigure}[t]{0.32\textwidth}
    \centering
    \includegraphics[width=\linewidth]{figs/kicad/4_erc_practice/4c913e30_step_78.png} 
    \caption{\small ERC reports only the three expected undriven-power errors for the external supplies, with zero warnings. The schematic is saved.}
    \label{fig:4c913e30_step_78}
   \end{subfigure}
  \caption{\small Task 4c913e30: opens ERC, dialog, results. }
  \label{fig:4_erc_practice_4c913e30}
\end{figure*}

\begin{figure*}[ht]
  \centering
  \begin{subfigure}[t]{0.32\textwidth}
    \centering
    \includegraphics[width=\linewidth]{figs/kicad/4_erc_practice/5dbc9e02_step_68.png} 
    \caption{\small The visible values, polarities, and seven nets match the design; no feedback errors appear. }
    \label{fig:5dbc9e02_step_68}
  \end{subfigure}
  \begin{subfigure}[t]{0.32\textwidth}
    \centering
    \includegraphics[width=\linewidth]{figs/kicad/4_erc_practice/5dbc9e02_step_69.png} 
    \caption{\small The saved title and status bar confirm the schematic’s location. ERC is ready.  }
    \label{fig:5dbc9e02_step_69}
   \end{subfigure}
   \begin{subfigure}[t]{0.32\textwidth}
    \centering
    \includegraphics[width=\linewidth]{figs/kicad/4_erc_practice/5dbc9e02_step_70.png} 
    \caption{\small ERC reports two expected undriven-power errors and zero warnings; no unconnected pins are reported. }
    \label{fig:5dbc9e02_step_70}
   \end{subfigure}
  \caption{\small Task 5dbc9e02: opens ERC, dialog, results. }
  \label{fig:4_erc_practice_5dbc9e02}
\end{figure*}

\begin{figure*}[ht]
  \centering
  \begin{subfigure}[t]{\textwidth}
    \centering
    \includegraphics[width=\linewidth]{figs/kicad/1_netlist_export_copied/a6414tw4_steps_06-10.png} 
    \caption{\small Current task: \texttt{a6414tw4} }
    \label{fig:a6414tw4_steps_06-10}
   \end{subfigure}

   \begin{subfigure}[t]{\textwidth}
    \centering
    \includegraphics[width=\linewidth]{figs/kicad/1_netlist_export_copied/4c913e30_steps_78-82.png} 
    \caption{\small Retrieved experience from an earlier task: \texttt{4c913e30}}
    \label{fig:4c913e30_steps_78-82}
  \end{subfigure}


  \caption{\small \textbf{Cross-task reuse of episodic memory in KiCad.} \textbf{Top:} Interaction with the current task (\texttt{a6414tw4}).
\textbf{Bottom:} The agent retrieves an earlier task (\texttt{4c913e30}) with a nearly identical action sequence: save the blank schematic, navigate to \emph{Export} $\rightarrow$ \emph{Netlist}, select the native KiCad format, and specify the output path. 
The retrieved episode provides a concrete precedent for this task. 
}
  \label{fig:kicad-cross-task-reuse}
\end{figure*}


% \subsection{Additional Related Works}
