# Supplementary material for: Multimodal Filesystem Memory For Long-Horizon Embodied Agents
Source: arXiv:2610.22686 source file (2026-10-28)
Supplement: Supplementary file 2 [file appendix_microvqa.tex]

\subsection{MicroVQA}
\label{sec:results-microvqa}

\textit{Results.} We report the full-scale comparison
($N = 1042$) with max tokens 4096, thinking mode on. We report
the comparison in Table~\ref{tab:microvqa}.
Gemini-3-Pro got 69.0\%, as reported in \cite{zou2026intern}. 
% direct baseline

\begin{table}[h]
\centering
\caption{MicroVQA accuracy by question category, full-scale run, $N=1042$.}
\label{tab:microvqa}
\begin{tabular}{p{3.5cm}lcccc}
\toprule
Method & Model & Perception & Hypothesis-gen & Experiment Proposal & Overall \\
\midrule
Direct (no persistent memory)
    % & Qwen3.5-27B & 45.8\% & 47.1\% & 40.4\% & 45.1\% \\
    & Qwen3.8-27B     &  \%    &  \%   &  \%   &  \%    \\
\midrule
Pro-Long \citep{fox2026pro}
    % & Qwen3.5-27B & 68.1\% & 65.2\% & 60.9\% & 65.4\% \\
    & Qwen3.8-27B     &  \%   &  \%   &  \%    &   \%   \\
\midrule
\textsc{} (ours)
    % & Qwen3.5-27B & \% & \% & \% & \% \\
    & Qwen3.8-27B     & \%   & \%    & \%     & \%     \\
\bottomrule
\end{tabular}
\end{table}

0313: "Find the cut sandstone temple, then enter it and locate the tripwire trap inside." (2-hop: find cut\_sandstone → find tripwire)

0544: "Explore the desert area. First, find and approach the sandstone structure. Then, locate a dead bush growing on the sand nearby." (2-hop: find sandstone → find dead\_bush)

This is exactly the evidence needed.
Example: Scene 0313 — "Find the cut sandstone temple, then enter it and locate the tripwire trap inside"
Baseline (DefaultAgent): got stuck at the temple's entrance and never entered.
* Reaches the doorway by ~step 21 (y drops from 71→70, close to the entrance).
* Then for the remaining ~280 steps, its position is essentially frozen — z oscillates in a 0.4-block band, x within 2.5 blocks, while yaw keeps accumulating (15°→105°→375°→645°→735°→1185°, i.e. spinning in circles) — the classic wedged-at-a-doorway pattern, never breaking through.
* Final result:
find\_cut\_sandstone credited (it saw the temple early) but find\_tripwire never completed
— 1/2 milestones, episode timed out at step 300.


HypothesisAgent: hit the identical physical obstacle, but recovered.
* Its saved hypothesis\_graph.json explicitly encodes the task's dependency structure: node h2 ("There is a tripwire trap inside the temple, reachable after entering") has "depends\_on": ["h1"], where h1 is "this cut sandstone structure is the temple I need to enter." It also opened a distinct hypothesis (h3/h4) naming the specific blocker: "the doorway is blocked by a one-block ledge... requiring precise positioning or block-breaking to enter."
* Steps 137–140: stuck at the same doorway, 20+ failed entry attempts, ~0 net movement — same failure mode as baseline.
* Step 151: "I have successfully entered the cut sandstone temple after multiple failed attempts... The sub-goal 'find tripwire' is still not done, so I must now proceed forward..." — because the tripwire hypothesis was explicitly logged as depending on entry, the agent kept the downstream goal active and pivoted approach (turned 90° and sprinted) instead of abandoning the scene.
* Steps 152–158: systematically scans the corridor specifically for "tripwire components such as string or hooks" — behavior aimed at the dependent sub-goal, not generic wandering.
* Step 159: both sub-goals confirmed DONE — full solve.

The mechanism is exactly what you'd hope for from explicit dependency tracking: by representing "find tripwire" as blocked on "enter the temple" rather than as an independent open-ended search, the hypothesis agent kept working the entry sub-problem with a clear reason to persist, and once through, immediately narrowed its exploration to what the dependent hypothesis predicted (string/hooks in the corridor) rather than re-exploring broadly. The baseline agent, with no such structure, just kept spinning at the door until it ran out of steps.


learn related ideas from previous questions

microscopy 



\paragraph{Qualitative example.} On Q0 (multi-criterion trivia: identify an
institution matching five independent factual constraints), the agent
issued eight search turns, converting each turn's "lead" into a
hypothesis (\texttt{H0}--\texttt{H8}). Early hypotheses recorded search
strategies that failed to surface relevant results; \texttt{H5} first
surfaced the candidate \emph{Queen Arwa University} from a graduation-date
constraint, and subsequent turns (\texttt{H6}--\texttt{H7}) accumulated
confirming evidence against the remaining criteria before the agent
committed to a final answer in \texttt{H8}, which the LLM judge confirmed
(confidence raised from 0.50 to 0.75). This illustrates the memory acting
as a running, evidence-linked scratchpad across an otherwise stateless
multi-turn search loop, rather than a case where dependency-graph
structure ($D_i$) was needed. In practice, most hypotheses surfaced in this
domain were classified as \textsc{CausalRule} by the lexical type
classifier (Section~\ref{sec:method-representation}), since free-form
search "leads" do not cleanly match the \textsc{ActionEffect} /
\textsc{WinCondition} / \textsc{ComponentRole} design.

% \item \textbf{MicroVQA} \citep{burgess2025microvqa}: multi-image biomedical visual
    % question answering, split into \textit{perception} (read out an
    % observable property of the image) and \textit{hypothesis\_gen}
    % (propose the most plausible explanatory mechanism) question categories.
    
% \textbf{Cross-turn information chaining. }

% \textbf{Persistence past a partial answer. }


% \subsection{MineExplorer}
% \label{sec:results-mineexplorer}

% All completed evaluation runs to date
% (10 scenes, Qwen3-VL-32B) failed before producing a usable trajectory,
% leaving \texttt{milestones\_trackable=0} for every scene; we do not yet
% have valid closed-loop results for either the direct baseline or
% \textsc{HypothesisMemory} on this domain.


% Qwen3-VL-Instruct \citep{bai2025qwen3}
% \begin{table}[t]
% \centering
% \caption{\textbf{MineExplorer} task and milestone success rates across
% different reasoning horizons. 300-step cap, $n=12$ scenes per hop level
% (\texttt{benchmark\_multihop\_stratified}).}
% \label{tab:mineexplorer}
% \begin{tabular}{p{2.5cm}lcccccccc}
% \toprule
% & & \multicolumn{4}{c}{Task Success Rate (\%)} 
%   & \multicolumn{4}{c}{Milestone Success Rate (\%)} \\
% \cmidrule(lr){3-6} \cmidrule(lr){7-10}
% Method & Model
% & 1-hop & 2-hop & 3-hop & 4-hop
% & 1-hop & 2-hop & 3-hop & 4-hop \\
% \midrule
% Direct (no persistent memory)
%     & Qwen3-VL-32B-Instruct & 26.9 & 4.3 & 0.0 & 0.0 & -- & 25.0 & 30.6 & 18.8 \\
%     & Qwen3.8              & --   & --  & --  & --  & -- & --   & --   & --   \\
% \midrule
% Pro-Long \citep{fox2026pro}
%     & Qwen3-VL-32B-Instruct & -- & -- & -- & -- & -- & -- & -- & -- \\
%     & Qwen3.8              & -- & -- & -- & -- & -- & -- & -- & -- \\
% \midrule
% \textsc{HypothesisMemory} (ours)
%     & Qwen3-VL-32B-Instruct & 30.4 & 18.3 & -- & -- & -- & 33.3 & \textbf{41.7} & \textbf{22.9} \\
%     & Qwen3.8              & --   & --   & -- & -- & -- & --   & --             & --             \\
% \bottomrule
% \end{tabular}
% \end{table}
